# Supplementary material for: InSpectre: Breaking and Fixing Microarchitectural Vulnerabilities by Formal Analysis
Source: arXiv:1911.00868 source file (2020-08-17)
Supplement: Supplementary file 1 [file appendix-short.tex]

\section{Theorem~\ref{thm:ooo:co}: Memory Consistency for OOO Semantics }
To show that $\doublestep{}{×}$ and $\singlestep{}{}$ are memory consistent we
prove a reordering lemma, which allows 
commuting transitions
if $(n+1)$-th transition modified  name $t_2$, 
$n$-th transition modified name $t_1$, and $t_2 < t_1$.
\vspace*{-0.7cm}
\begin{center}
\begin{tikzpicture}[node distance=2cm,auto,>=latex']
\tikzstyle{every node}=[font=\small]
\tikzset{pblock/.style = {rectangle, draw=white!50, top
                      color=white,bottom color=white, align=center, minimum width=1cm}}
\node[pblock,name=a1]{$\newstate_1$};                      
\node[pblock,name=a2, right of  = a1]{$\newstate_2$};
\node[pblock,name=a3, right of  = a2]{$\newstate_n$};
\node[pblock,name=a4, right of  = a3]{$\newstate_{n+1}$};
\node[pblock,name=a4', below = 0.5cm of a4]{$\newstate'_{n+1}$};
\node[pblock,name=a5, right of  = a4]{$\newstate_{n+2}$};
\draw[->]  (a1) edge  node[above] {} (a2);
\draw[->]  (a2) edge[dashed]  node[midway,sloped,rotate=90]{} (a3); 
\draw[->]  (a3) edge node[above,sloped] {$(\alpha_1, t_1)$}  (a4);
\draw[->]  (a4) edge node[above,sloped] {$(\alpha_2, t_2)$}  (a5);
\draw[->]  (a3) edge node[below left] {$(\alpha_2, t_2)$}  (a4');
\draw[->]  (a4') edge node[below right] {$(\alpha_1, t_1)$}  (a5);
\end{tikzpicture}
\end{center}

\emph{Notation:} For a sequence of states
$\newstate_0 \dots \newstate_n$,
we define $(\Inst_j, \storage_j, \commits_j, \decodes_j) = \newstate_j$ 
for $i \in \{0 \dots n\}$,
$(\alpha_i, t_i) = \stepparam(\newstate_{i-1}, \newstate_{i})$
and $(\Inst_{i-1} \cup \hat{\Inst}_{i}, \storage_{i-1} \cup \hat \storage_{i},
\commits_{i-1} \cup \hat \commits_{i}, \decodes_{i-1} \cup \hat \decodes_{i}) =
(\Inst_{i}, \storage_{i}, \commits_{i}, \decodes_{i})$ for $i \in
\{1 \dots n\}$.

We first show that $\strfor$s and $\stract$s of 
$t$ do not depend on names greater than $t$ and  are monotonic.
\begin{lemma}\label{lemma:activestore:reorder}
  Let $\newstate_0$ and $\newstate_1$ be two states, 
  if $bn(\hat \Inst_1) \geq t$ and $\dom{\hat \storage_i} \geq t$ then
  $\strfor(\newstate_1,t) = \strfor(\newstate_0,t)$ and
  $\stract(\newstate_1, t) =  \stract(\newstate_0, t)$
\end{lemma}
\begin{proof}
Let $t$ be a load or store accessing address $t_a$ (the other cases are
trivial, since $\stract$ is undefined), hence $t_a < t$.\\
(1) The instructions that precede $t$ are the same in $\newstate_0$ and
$\newstate_1$. 
(2) For every store that precedes $t$, the evaluation of condition and
address is the same in $\newstate_0$ and $\newstate_1$, since they can only
reference names smaller than $t$.
% let $\iota' = \ass{c'}{t'}{\store{\restype}{t'_a}{t'_v}}$ and $t' < t$
% then $n(c') \cup \{t'_a\} < t$. Therefore, $\den{c'}{\storage_0 \cup
% \hat \storage_1} = \den{c'}{\storage_0}$ and $(\storage_0 \cup
% \hat \storage_1)(t'_a) = \storage_0(t'_a)$.\\
(3) % Similarly, since $t_a < t$ then
$(\storage_0 \cup
\hat \storage_1)(t_a) = \storage_0(t_a)$.\\
Properties (1, 2, 3) guarantee that $\strfor(\newstate_1,t) =
\strfor(\newstate_0,t)$. Similarly, since $\stract$ depends on the
addresses and conditions of stores in $\strfor(\newstate_1,t)$ and these have 
names smaller than $t$ then
$\stract(\newstate_1,t) =
\stract(\newstate_0,t)$.
\end{proof}
\vspace*{-0.5cm}
\begin{lemma}\label{lemma:pas:mono}
  if $\newstate_0 \doublestep{l}{} \newstate_1$ and $\ass{c}{t}{o} \in \newstate$ then
  $\strfor(\newstate_1, t) \subseteq \strfor(\newstate_0, t)$ and
  $\stract(\newstate_1, t) \subseteq \stract(\newstate_0, t)$
\end{lemma}
\begin{proof}
  The proof is by cases analysis on $\alpha_1$.
  For commits the proof is trivial, since $\hat \Inst_1 =
  \emptyset$ and $\hat \storage_1 = \emptyset$.
  For fetches, $\hat \storage_1 = \emptyset$ and the transition may decode new
  stores in $\hat \Inst_1$. However, these new stores
  have names greater than $max(\Inst_0)$, hence their names are greater than
  $t$. Therefore the additional stores do not affect $\strfor$ and 
  $\stract$.
  
  For executions, $\hat \Inst_1 = \emptyset$, $\hat \storage_1 =
  \{t_1 \mapsto v\}$, and $\fundefined{\storage_0}{t_1}$ for some $v$.
  This store update can make defined the evaluation of the
  condition or expression of a store. In this case, if a store is in
  $\strfor(\newstate_1, t)$ it must also be in $\strfor(\newstate_0, t)$.
  % Stores that are in $\strfor(\newstate_0, t)$ but are not in
  % $\strfor(\newstate_1, t)$ have undefined condition or address in
  % $\newstate_0$ and false condition or non matching address in $\newstate_1$.\\
  To show that $\stract$ does not increase we proceed as follows.
  Let $t'$ be a store in $\strfor(\newstate_0, t) \setminus
  \stract(\newstate_0, t)$.
  There must be a subsequent overwriting store $t''$ in $\strfor(\newstate_0, t)$
  whose condition holds in $\newstate_0$ and address is defined in
  $\newstate_0$.
  Such store cannot have $t_1$ in its free names, hence it is also in
  $\strfor(\newstate_1, t)$. Therefore the store $t''$ overwrites $t'$ in
  $\newstate_1$ too.
\end{proof}
Proof of Theorem~\ref{thm:ooo:co} is done by induction on the length
of traces and relies on Lemma~\ref{lemma:switch-pre} to demonstrate
that $(\alpha_2, t_2)$ can be applied in $\newstate_n$ and
Lemma~\ref{lemma:switch-post} to show that $(\alpha_1, t_1)$ can be
applied in the resulting state $\newstate'_{n+1}$ to obtain
$\newstate_{n+2}$.
\begin{lemma}\label{lemma:switch-pre}
If $\newstate_0 \doublestep{l_1}{} \newstate_1 \doublestep{l_2}{} \newstate_2$ and 
$t_2 < t_1$ then $\newstate_0 \doublestep{l_2}{}
(\Inst_{0} \cup \hat \Inst_{2}, \storage_{0} \cup \hat \storage_{2},
\commits_{0} \cup \hat \commits_{2}, \decodes_{0} \cup \hat \decodes_{2}) =
\newstate'$,
$\stepparam(\newstate_0, \newstate') = (\alpha_2, t_2)$, and if $\alpha_2 =
\cmt(a, v)$ then $\alpha_1 \neq \cmt(a, v')$.
\end{lemma}
The proof that $t_2$ can be executed in $\newstate_0$ (i.e., $\alpha_2=\exe$) relies on
the fact that all free names of the instruction $t_2$ are smaller
than $t_2$. Therefore% , since $t_2 < t_1$,
the evaluation of expressions
and condition of the instruction $t_2$ is the same in $\newstate_{0}$ and
$\newstate_{1}$. For the same reason, if $t_2$ is a load,
Lemma~\ref{lemma:activestore:reorder} guarantees that
$\stract(\newstate_0, t_2) = \stract(\newstate_1, t_2)$. These properties guarantee
that the denotation semantics of $t_2$ is the same in
$\newstate_{0}$ and $\newstate_{1}$. The same Lemma is used to show that
$t_2$ can be committed or fetched in $\newstate_0$ (i.e., $\alpha_2=\cmt$
or $\alpha_2=\ftc$), since
$t_1 > t_2$ then $\newstate_0(t_2)=\newstate_1(t_2)$ and $\alpha_1$ cannot commit or fetch a store that
overwrite the update of $t_2$.
For fetches (i.e, $\alpha_2=\ftc$), since intructions are fetched in
program order, it also holds that $\alpha_1 \neq \ftc$ and
$\hat \Inst_{1} = \emptyset$.
This guarantees that $max(\Inst_0) = max(\Inst_1)$ and therefore
fetching $t_2$ in $\newstate_0$ produces the same MIL translation of
$\newstate_1$.

\begin{lemma}
  \label{lemma:switch-post}
  If $\newstate_0 \doublestep{l_1}{} \newstate_1 \doublestep{l_2}{} \newstate_2$
  and $t_2 < t_1$ then exists $\newstate'$
 such that
 $\newstate_0 \doublestep{l_2}{} \newstate' \doublestep{l_1}{} \newstate_2$,
 $\stepparam(\newstate_0, \newstate') = (\alpha_2, t_2)$,
  $\stepparam(\newstate', \newstate_2) = (\alpha_1, t_1)$,
  and if $\alpha_2 = \cmt(a, v)$ then $l_1 \neq \cmt(a, v')$.
\end{lemma}
The existence of $\newstate'$ is given by Lemma~\ref{lemma:switch-pre}.
The proof to show that $t_1$ can be executed (i.e., $\alpha_1=\exe$)
from $\newstate'$ is trivial if $\alpha_2 \neq \exe$.
If $\alpha_2=\exe$ then $\fundefined{\newstate_0}{t_2}$. Since $\exe$ is enabled in $\newstate_0$,
then $t_2$ is not in the free names of $t_1$.
This and Lemma~\ref{lemma:pas:mono} guarantee that if $\den{\cdot}$ of $t_1$
in $\newstate_0$ is $(v, l_1)$ then exists $l'_1$ such that $\den{\cdot}$ of $t_1$
in $\newstate'$ is $(v, l')$.
Notice that for internal operations and
stores $l'_1 = l_1 = \cdot$. For loads, either 
$l'_1= l_1 = \dl a$ or $l'_1= \dl a$ and $l'_1= \cdot$. The latter
happens when $\stepparam(\newstate_0, \newstate') = (\cmt(a, v), t_2)$. % In
% this case, we have reordered a memory commit before a load thus
% making it impossible to forward the value of the store to the load
% and requiring a new memory interaction. 
This shows that the
observations of the OOO model are a subset of the
observations of in-order model, since the OOO model 
can execute loads before the corresponding stores are committed.
For case of commits and fetches (i.e., $\alpha_1=\cmt$ or
$\alpha_1=\ftc$) the proof relies on Lemma~\ref{lemma:pas:mono} and
the fact that commits for the same address and fetches are done in
program order (i.e. $\bn(\strfor(\newstate_0, t_1)) \subseteq \commits_0$
and $\bn(\strfor(\newstate_0, t_1)) \subseteq \decodes_0$), hence $\alpha_2$
cannot be a colliding commit or fetch.

\section{Lemma~\ref{lem:deps-eq}: Proof of correctness of $t$-equivalence }
  If $\newstate_1  \sim_t  \newstate_2$ and the $t$'s microinstruction  
  in $\newstate_1$ is $\instr = \ass{c}{t}{o}$, then
  $\deps(t, \newstate_1) = \deps(t, \newstate_2)$,
  $\den{c}\newstate_1 = \den{c}\newstate_2$,
  and if $\den{\inst}\newstate_1 = (v_1, l_1)$ and $\den{\inst}\newstate_2 =
  (v_2, l_2)$ then $v_1 = v_2$. 

  \begin{proof}
    For non-load operations and guards the proof is trivial, since their semantics only
  depends on the value of the bound names of the operation and
  guard. % These names are statically identified from $c$ and $o$ and their value is the same in $\newstate_1$ and
  % $\newstate_2$ by definition of $\sim_t$.
  For loads, the proof relies on
  showing that for every state $\newstate$, 
  $\stract(\newstate, t)
  =
  \stract(\proj{\newstate}{T}, t)
  $, where $T=\deps(t, \newstate)$.
  Let $t' \in \stract(\newstate, t)$. By
  definition, $t'$ and its bound names are in $T$, therefore their
  values are equal in $\newstate$ and $\proj{\newstate}{T}$ and hence $t'
  \in \strfor(\proj{\newstate}{T},t)$. Also, by definition of
  $\deps$, all names referred by conditions and addresses of
  subsequent stores of $t'$ are in $T$. Therefore
  if there is no subsequent store
  that overwrites $t'$ % (i.e.,  $\ass{c''}{t''}{\store{\restype}{t''_a}{t''_v}}$ such that 
  % $[c'']\newstate$ and $(\newstate(t''_a) = \newstate(t) \vee
  % \newstate(t''_a) = \newstate(t_a))$)
  then
  there is no store overwriting $t'$ in  $\proj{\newstate}{T}$ and
  hence $t' \in \stract(\proj{\newstate}{T}, t)$.
\end{proof}
\vspace*{-0.5cm}
\newcommand{\ctbisimrel}{\mathbf{R}}
\section{Theorem~\ref{thm:ct}: Proof of Security of MIL Constant Time}
The proof demonstrates that the relation $\ctbisimrel$ is a bisimulation for the
OOO transition relation, where $\newstate \ctbisimrel \newstate'$
iff $\newstate \bisim \newstate'$ and exist $\newstate_0 \sim_L
  \newstate'_0$ and $n$ such that $\newstate_0 \doublestep{}{}^n \newstate$ and $\newstate'_0
  \doublestep{}{}^n \newstate'$.

Let $(\Inst, \storage, \commits. \decodes) = \newstate$,
$(\Inst', \storage', \commits'. \decodes') = \newstate'$,
$\newstate \doublestep{l}{} \newstate_1 = (I \cup \hat I, \storage \cup \hat \storage, \commits
\cup \hat \commits, \decodes \cup \hat \decodes)$, and $\stepparam(\newstate,
  \newstate_1) = (\alpha, t)$.
The proof is done by cases on $\alpha$. We detail the case for
$\alpha=\exe$, since the other cases are similar.

The hypothesis of the rule ensure that 
$\inst = \ass{c}{t}{o} \in \Inst$,
  $\fundefined{\storage}{t}$,  $\den{c}{\storage}$, and
  $\den{\inst}\newstate = (v, l)$.
  The conclusion of the rule ensures that $\hat \storage = \{t \mapsto v\}$,
  $\hat \commits=\emptyset$, $\hat \decodes=\emptyset$, and
  $\hat \Inst = \emptyset$.\\
  Relation $\bisim$ ensures that  $\inst \in \Inst'$,
  $\fundefined{\storage'}{t}$,  and $\den{c}{\storage'}$.

  We must show that exists $v'$ such that $\den{\inst}\newstate' = (v', l)$.
  For $o = e$ and $o = \store{\restype}{t_a}{t_v}$ the proof is trivial. In fact,
  since $\den{\inst}\newstate$ then all free names of $o$ are defined in
  $\newstate$ and $\bisim$ ensures that the same names are defined in
  $\newstate'$.
  For $o = \load{\restype}{t_a}$, $\den{\inst}\newstate = (v, l)$ ensures
  that $\bn(\stract(\newstate, t)) = \{t_s\}$, $\fdefined{\newstate}{t_a}$, and
  $\fdefined{\newstate}{t_s}$. Relation $\bisim$ ensures that
  $\newstate'(t_a)=\newstate(t_a)$, $\fdefined{\newstate'}{t_s}$,
  $\Inst=\Inst'$ (hence they are the same 
  instruction), and that for every store
  $\ass{c'}{t'}{\store{\restype}{t'_a}{t'_v}}$,
  $\den{c'}\newstate=\den{c'}{\newstate'}$, and
  $\newstate(t'_a)=\newstate'(t'_a)$. Therefore
  $\bn(\stract(\newstate', t)) = \bn(\stract(\newstate, t))$
  and $\den{\inst}\newstate' = (\newstate'(t_s), l')$. Finally, since
  relation $\bisim$ guarantees that $(t_s \in \commits) \Leftrightarrow
  (t_s \in \commits')$ then $l'=l$.
  \\
  These properties permit to apply rule ($\exe$) to show that
  $\newstate' \doublestep{l}{} (\Inst', \storage' \cup \{t \mapsto \storage'(t_s)\}, \commits',
  \decodes') = \newstate'_1$.
  \\
  To prove that $\bisim$ is preserved we leverage on 
  Theorem~\ref{thm:ooo:co}.
  Let $\ass{c'}{t'}{o'} \in \Inst$. Let $\ANames'$ be $fn(c')$ if 
  $o'$ is neither a load or a store; $fn(c') \cup
  \{t'_a\}$ if $o'$ is a memory or register access and $t'_a$ is the
  corresponding address;
  $fn(c') \cup
  \{t'_v\}$ if $o'$ is a PC update and $t'_v$ is the
  corresponding value.
  If $t \not \in \ANames'$ then the proof is trivial, since
  $\den{c}{\storage \cup \{t  \mapsto v\}} = \den{c}{\storage} =
  \den{c}{\storage'} = \den{c}{\storage' \cup \{t  \mapsto
    \storage'(t_s)\}}$ (similarly for the address in case of a
  resource accesses or PC update).

\begin{center}
\begin{tikzpicture}[node distance=2cm,auto,>=latex']

\tikzstyle{every node}=[font=\small]
\tikzset{pblock/.style = {rectangle, draw=white!50, top
                      color=white,bottom color=white, align=center, minimum width=0.75cm}}
                      
\node[pblock,name=a1]{$\newstate_0$};                      
\node[pblock,name=a2, right of  = a1]{$\newstate$};
\node[pblock,name=a3, right of  = a2]{$\newstate_1$};
\node[pblock,name=a4, right of  = a3]{$\newstate_{S}$};
                
\node[pblock,name=a'1, below = 0.4cm of a1]{$\newstate'_0$};                      
\node[pblock,name=a'2, right of  = a'1]{$\newstate'$};
\node[pblock,name=a'3, right of  = a'2]{$\newstate'_1$};
\node[pblock,name=a'4, right of  = a'3]{$\newstate'_{S}$};

\draw[->]  (a1) edge[dashed]  node[above] {$n$} (a2);
\draw[->]  (a2) edge  node[above]{$(\alpha, t)$} (a3); 
\draw[->]  (a3) edge[dashed] node[above,sloped] {$m$}  (a4);
\draw[->]  (a1) edge[dashed,bend left=20]  node[above] {$n+1+m$} (a4);

\draw[->]  (a'1) edge[dashed]  node[above] {$n$} (a'2);
\draw[->]  (a'2) edge  node[midway,sloped]{} (a'3); 
\draw[->]  (a'3) edge[dashed] node[above,sloped] {$m$}  (a'4);
\draw[->]  (a'1) edge[dashed,bend right=15]  node[below] {$n+1+m$} (a'4);

\draw[-]  (a1) edge  node[left] {$\sim_L$} (a'1);
\draw[-]  (a2) edge  node[left] {$\ctbisimrel$} (a'2);
\draw[-]  (a4) edge  node[left] {$\bisim$} (a'4);
\draw[-]  (a3) edge  node[left] {$\ctbisimrel$} (a'3);
\end{tikzpicture}
\end{center}
\vspace*{-0.3cm}
For $t \in fn(c')$ we reason as follows.
States $\newstate_1$ and
  $\newstate'_1$ are the $(n+1)$-th states of two
  OOO traces $\rho = \newstate_0 \doublestep{}{}^{n+1} \newstate_1$ and $\rho' = \newstate'_0 \doublestep{}{}^{n+1} \newstate'_1$ such that $\newstate_0
  \sim_{L} \newstate'_0$.
  \todo{There is?} There is a trace $\rho_1 = \newstate_0 \doublestep{}{}^{n+1}
  \newstate_1 \doublestep{}{}^{m} \newstate_s$ that has
  prefix $\rho$, such that $\completed{\newstate_s, t''}$
  for every $t'' \leq max(bn(\Inst'))$. Notice that this state is ``sequential''.
  Since in the OOO semantics the storage is monotonic  then
  $\newstate_1(t) = \newstate_s(t)$.
  Theorem~\ref{thm:ooo:co} relates this trace to a
  sequential trace, enableing to use the MIL constant-time hypothesis.
  In fact, there exists an ordered
  execution $\pi$ of $\rho_1$ that ends in $\newstate_s$: $\pi = \newstate_0 \singlestep{}{}^{n+1+m}
  \newstate_s$.
  For the same reason, $\rho'$ is a prefix
  of a trace $\rho'_1$ that ends in a sequential state $\newstate'_s$,
  $\newstate'_s(t) = \newstate'_1(t)$, and there exists a sequential trace $\pi'$
  of $n+1+m$ steps  that
  ends in $\newstate'_s$.
  Since $\completed{\newstate_s, t''}$ and $\completed{\newstate'_s, t''}$
  then $\fdefined{\den{c'}}{\newstate_s}$ and
  $\fdefined{\den{c'}}{\newstate'_s}$.
  Therefore, we can use the assumption on MIL constant-time to show
  that
  $\newstate_s \bisim \newstate'_s$, hence $\den{c'}{\newstate_s} = \den{c'}{\newstate'_s}$. Since $t \in fn(c)$,
  either $\fundefined{\den{c'}}{\newstate_s}$ and
  $\fundefined{\den{c'}}{\newstate'_s}$ or $\den{c'}{\newstate_1} =
  \den{c'}{\newstate'_1}$.
  Cases where $t'$ is a resource access and $t
  = t'_a$, or  $t'$ is PC update and $t
  = t'_v$ are similar.

\section{Theorem~\ref{thm:spec:co}: Memory Consistency   for Speculative Semantics }
\label{appendix:proof:spec:cho}
Since the OOO semantics
already takes care of reordering, to prove Theorem \ref{thm:spec:co} a
bisimulation argument between $\triplestep{}{}$ and $\doublestep{}{}$
suffices. Intuitively, referring to Figure \ref{fig:speculation},  
the states ``decoded'', ``guessed'', ``speculated'' and ``speculatively fetched'' in the speculative semantics  correspond 
to the state ``decoded'' in the OOO semantics, in that progress can still be undone to return to the ``decoded'' state.
Similarly, the state ``retired'' corresponds to ``executed'', ``fetched'' to ``fetched'' and ``committed'' to
``committed''. The only exception consists of speculatively
fetched. In this case there is an option to directly retire the
fetched microinstruction, without passing through ``retired'' first. The proof
reflects this intuition. 
 
%

%  The main challenges in defining the bisimulation are i) to pin down
%  the non-speculated instructions in the speculative semantics and
%  relate them correctly to instructions in the OOO semantics, and ii)
%  account for speculatively fetched instructions. The latter issue
%  arises when retiring an instruction in the speculative semantics that
%  has earlier been speculatively fetched. In that case, the
%  corresponding decoded microinstructions
%  are already in flight, although the bisimilar OOO state will have no
%  trace of this. 
%  Then the OOO microinstruction will have to be first executed and then
%  fetched. The following definitions make this intuition precise.

 To simplify our proof, without loss of generality, we impose that $\translate(v,t)=\Inst$ and $\ass{c}{t}{\store{\Pc}{}{t_v}} \in
 \Inst$ then $t \not \in fn(\Inst)$, there is no $\ass{c}{t'}{\load{\Pc}} \in I$ such
 that $t' < t$, and there is no $\ass{c}{t'}{\store{\Pc}{}{t'_v}} \in
 I$ and storage $\storage$ such that $\den{c}s \land \den{c'}s$ .
This  condition permits to uniquely identify the PC
store that generated a microinstruction.

We say that a name $t'$ is \emph{produced by} the PC store
$\ass{c}{t}{\store{\Pc}{}{t_v}}$, if $t' \prec
t$.
We extend this notion to set of microinstructions.
Say that $\Inst_1$
\emph{produces} $\Inst_2$, 
$\Inst_1<\Inst_2$, if there is $t \in \Inst_1$ such that for each
$t'\in\Inst_2$, $t'$ is produced by $t$.
Say then that $\Inst$ (and by extension states containing $\Inst$) is \emph{well-formed}
by the partitioning $\Inst_{retired},\Inst_1,\ldots,\Inst_n$, if
$\Inst=\bigcup\{\Inst_{retired},\Inst_1,\ldots,\Inst_n\}$,
$\Inst_{retired}$ is retired (i.e., $bn(\Inst_{retired}) \cap
\dom{\spec} = \emptyset$), and for each $\Inst_i$, $1\leq i\leq n$ there is
$\Inst\in\{\Inst_{retired},\Inst_1,\ldots,\Inst_n\}$ such that $\Inst
< \Inst_i$. We require that $<^*$ on the partitions
% $\{\Inst_{retired},\Inst_1,\ldots,\Inst_n\}$
is well-founded and the
partitions are maximal. % Observe that 
All reachable states  in the
speculative semantics are well-formed and each partition corresponds
to the translation of one single ISA instruction.
We say that an ISA instruction $\Inst_i$ in the
partitioning $\Inst_1,\ldots,\Inst_n$ is \emph{unconditionally
  fetched}, if $\Inst_{retired}< \Inst_i$ and let $\Inst_{uf}$ be the
union of $\Inst_{retired}$ and the 
instructions that have been unconditionally fetched.

We proceed to define the bisimulation $R$. We restrict attention to reachable states in both the OOO and speculative semantics in order to keep the definition of $R$ manageable and be able to implicitly make use of simple invariant properties. 
Let $(\Inst_1,  \storage_1, \commits_1, \decodes_1)\ R\  (\Inst_2,
\storage_2,  \commits_2, \decodes_2, \spec_2, \guesses_2) $ if 
\begin{inparaenum}[1.]
\item $\Inst_2$ is well-formed by the partitioning $\Inst_{2,retired},\Inst_{2,1},\ldots,\Inst_{2,n}$,
\item There is a bijection $\widetilde{\cdot}$ from $\Inst_{2,uf}$ to $\Inst_1$,
\item $\commits_2 = \widetilde{\commits_1}$,
\item $\mapminus{\storage_2}{\dom{\spec_2}} = \widetilde{\storage_1}$,
\item $\decodes_2 \setminus\dom{\spec_2} = \widetilde{\decodes_1}$.
%\item $\{  \ass{c}{t}{o} \in \Inst_2 \mid
%  \forall \ass{c'}{t'}{\store{\pc}{\_}{t'_v}} \in \Inst_2. t\prec t' \Rightarrow
%  %t' \in \dom{\spec_2(t)}\Rightarrow 
%  t' \not\in \dom{\spec_2}\} = \Inst_1$. 
\end{inparaenum}
In 3.-5. the bijection $\widetilde{\cdot}$ is pointwise extended to sets and expressions.

Note that, from 2. and 4. we get that a microinstruction
$\widetilde{t}$ in $\Inst_1$ has been executed iff
$\fdefined{\storage_2}{t}$ and $t\notin\dom{\spec_2}$.
We prove that $R$ is a weak bisimulation in two steps. We first show that all speculative transitions up until retire or non-speculative fetch are reversible. To prove this it is sufficient to show that each of the conditions 1.--4. is invariant under $\prd$, $\exe$, $\pexe$, $\rbk$, and $\ftc$, the latter under the condition that
the fetched instruction is in $\spec_2$. These transitions are
identified by $T1$ in the following picture:
\vspace*{-0.3cm}
\begin{center}
\begin{tikzpicture}[node distance=2.5cm,auto,>=latex']
\tikzstyle{every node}=[font=\small]
\tikzset{pblock/.style = {rectangle, draw=white!50, top
                      color=white,bottom color=white, align=center, minimum width=0.75cm}}
                      
\node[pblock,name=a1]{$(\newstate_2, \spec_2, \guesses_2)$};                      
\node[pblock,name=a2, right of  = a1]{$(\newstate'_2, \spec'_2, \guesses'_2)$};
\node[pblock,name=a3, right of  = a2]{$(\newstate''_2, \spec''_2, \guesses''_2)$};
\node[pblock,name=a4, right of  = a3]{$(\newstate'''_2, \spec'''_2, \guesses'''_2)$};
                
\node[pblock,name=a'1, below = 0.7cm of  a1]{$\newstate_1$};                      
\node[pblock,name=a'2, right of  = a'1]{$\newstate'_1$};
\node[pblock,name=a'3, right of  = a'2]{$\newstate''_1$};
\node[pblock,name=a'4, right of  = a'3]{$\newstate'''_1$};

\draw[->]  (a1) edge  node[above] {T1} (a2);
\draw[->]  (a2) edge  node[above]{T2} (a3); 
\draw[->]  (a3) edge  node[above]{T3} (a4); 

\draw[->]  (a'1) edge  node[above] {T2} (a'2);
\draw[->]  (a'2) edge  node[above] {\exe} (a'3);
\draw[->]  (a'3) edge  node[above] {\ftc} (a'4);

\draw[-]  (a1) edge  node[left] {$R$} (a'1);
\draw[-]  (a2) edge  node[left] {$R$} (a'1);
\draw[-]  (a3) edge  node[left] {$R$} (a'2);
\draw[-]  (a4) edge  node[left] {$R$} (a'4);
\end{tikzpicture}
\end{center}

%\todo[inline]{From here need to update proof to new bisimulation conditions. In particular $1\mapsto 3, 2\mapsto 4, 3\mapsto 5$, and 4 is replaced by the new 1,2}

\begin{lemma}
\label{lem:bisim:one}
If $\newstate_1\ R\ (\newstate_2,\spec_2,\guesses_2)$ and 
$(\newstate_2,\spec_2,\guesses_2)\triplestep{}{} (\newstate_2',\spec_2',\guesses_2')$ is an instance of $\prd$, $\exe$, $\pexe$,$\rbk$, or speculative $\ftc$ then $\newstate_1\ R\ (\newstate_2',\spec_2',\guesses_2')$.
\end{lemma}
\begin{proof}
  For $\prd$, $\exe$, $\pexe$ the proof is trivial, since the
  transition extends the storage with $t$ and adds $t$ to $\dom{\spec'_2}$ hence the transition does not affect the
  bisimulation.\\
  For $\rbk$, the transition removes $t$ from $\storage_2$ and
  $\spec_2$. If $t$ is not a PC store this has no effect in the
  bisimulation, since $t \in \dom{\spec_2}$.
  If $t$ \emph{is} a PC store
  then we need to observe the following: Since $t$ is speculated, $t$ is a member of some partition $\Inst_{2,i}$. The set
 $\Delta^+$ contains all partitions $\Inst_{2,j}$ such that $\Inst_{2,i}<^+ \Inst_{2,j}$. In particular, no such $\Inst_{2,j}$ is in $\Inst_{2,fu}$, since
 otherwise $\Inst_{2,j}$ would have been added by a retired PC store. It follows that the bijection $\widetilde{\cdot}$ is not affected by
 the removal of $\Delta^+$, and 1 and 2 are reestablished for the new
 speculative state. Similarly, condition 4 and 5 are reestablished
 because the removed instructions are all in $\dom{\spec_2}$.\\
 For $\ftc$ and $t \in \dom{\spec_2}$ we observe that no instruction added to $\Inst_2$ can
 belong to $\Inst_{2,fu}'$, since all such microinstructions are produced
 by a non-retired PC store microinstruction.
\end{proof}
The following Lemma handle cases for $\ret$ when $t \not \in
\decodes_2$, $\cmt$, $\ftc$ when $t \not \in \dom{\delta_2}$ (which
are identified by $T2$ in Figure), and the cases for 
$\ret$ when $t \in \decodes_2$ (which
are identified by $T3$ in Figure).

\todo{We never talk about step param that is needed for seq consistency}
\begin{lemma}
\label{lem:bisim:two}
Assume that $\newstate_1\ R\ (\newstate_2,\spec_2,\guesses_2)$.
\begin{enumerate}
\item
If $(\newstate_2,\spec_2,\guesses_2)\triplestep{}{}(\newstate_2',\spec_2',\guesses_2')$ is an instance of $\cmt$, $\ftc$, or $\ret$ then 
$\newstate_1 \doublestep{}{}^{\ast}\newstate_1'$ such that $\newstate_1'\ R\ (\newstate_2',\spec_2',\guesses_2')$.
\item
If $\newstate_1 \doublestep{}{}\newstate_1'$ then $(\newstate_2,\spec_2,\guesses_2)\triplestep{}{}(\newstate_2',\spec_2',\guesses_2')$
such that $\newstate_1'\ R\ (\newstate_2',\spec_2',\guesses_2')$.
\end{enumerate}
\end{lemma}
\begin{proof}
  We sketch the proof for
  $(\newstate_2,\spec_2,\guesses_2)\triplestep{}{}(\newstate_2',\spec_2',\guesses_2')$.
  The converse direction is straightforward.
  
  The case for $\cmt$ and $\ftc$ when $t \not \in
  \dom{\delta_2}$ are straightforward. Since $t\notin\dom{\spec_2}$
  we get $\storage_1(\widetilde{t}) = \widetilde{v}$ by cond. 4,
  $\widetilde{t} \notin \widetilde{\commits_1 \cup \decodes_1}$ by
  cond. 3 and 5,
  $\widetilde{t}\in\widetilde\Inst_2$ by cond. 2, and, 
since all members of $\bn(\strfor(\newstate_2, t))$ are non-speculated,
by cond. 2, 3, 4, $\bn(\strfor(\newstate_1, \widetilde{t})) \subseteq
\commits_1 \cup \decodes_1$. In case of $\ftc$ the bijection
$\widetilde \cdot$ can be trivially extended to cover the newly decoded
microinstructions. It follows that the OOO can perform the
same transition and establish conditions 1.-5.

The case for $\ret$ when $t \not \in
\decodes_2$ relies on $t$-equivalence.
Let $\inst = \ass{c}{t}{o}$ be the
microinstruction bound to $t$ in $\Inst_2$.
The hypothesis of the transition rule ensure that
$t\in\dom{\storage_2}$, $\dom{\spec_2(t)}\cap \dom{\spec_2}
=\emptyset$, and $(\Inst_2,\storage_2,\commits_2,\decodes_2) \sim_t
(\Inst_2,\spec_2(t),\commits_2,\decodes_2)$.
Therefore $\den{\inst}{(\Inst_2,\storage_2,\commits_2,\decodes_2)} = \storage_2(t)$.
The conclusion  ensures that $\Inst_2'=\Inst_2$, 
$\storage_2' =\storage_2$, $\commits_2'=\commits_2$, $\decodes_2'=\decodes_2$, $\spec_2'=\proj{\spec_2}{\overline{\{t\}}}$, and
$\guesses_2'=\guesses_2$.
 Since
$\dom{\spec_2}\cap\dom{\spec_2(t)}=\emptyset$ we know that
$t\in\Inst_{2,uf}$ and hence $\widetilde{t}\in\dom{\Inst_1}$ by 2.
 It follows that $\widetilde{t}$ can be executed from $\newstate_1$
 resulting in $\newstate'_1$, where $\Inst_1'=\Inst_1$, $\storage_1' = \storage_1[\widetilde{t}\mapsto \storage_2(t)]$
such that $\storage_1'(\widetilde{t}) = \widetilde{\storage_2'(t)}$, $\commits_1'=\commits_1$, and $\decodes_1'=\decodes_1$. This suffices to
reestablish $R$.

The case for $\ret$ when $t \in \decodes_2$ we must additionally
consider the microinstructions produced by $t$, i.e., the partition
$\hat \Inst_{2}$ of $\Inst_2$ such that $\{\ass{c}{t}{o}\} < \hat
\Inst_{2}$. These are not in $\Inst_{2,uf}$, since $t
\in \dom{\spec_2}$, hence are not covered by the bijection $\widetilde \cdot$.
However, microinstructions in $\hat \Inst_{2}$ are in $\Inst'_{2,uf}$.
Therefore,  to restablish the bisimulation, the OOO must
perform another step from $\newstate'_1$ applying $\ftc$ to $t$. 
This allows extending the bijection  
$\widetilde \cdot$ to relate the newly decoded
microinstructions to $\hat \Inst_{2}$.

\end{proof}

\section{Other Countermeasures}
\subsection{Retpoline for Spectre-BTB}

A known countermeasure to Spectre-BTB is the \emph{Retpoline} technique developed by Google~\cite{retpoline}. 
In a nutshell, retpolines are instruction snippets that isolate indirect jumps from speculative execution
via call and return instructions.
% \emph{Retpoline} counters Spectre-BTB by emulating indirect jumps 
% via call and return instructions. 
% The following MIL program models a single indirect
% branch which (cf. Section~\ref{sec:spectre:btb}) is vulnerable to Spectre-BTB:
% \begin{center}
% \begin{tikzpicture}[node distance=3.5cm,auto,>=latex']
% \pomsetstyle
% \picloadT{t_1}{\Regs}{r_{11}}
% \picexpT[right of = t_1]{t_2}{t_1}
% \picstoreT[right of = t_2]{t_3}{\pc}{}{t_2}
% \draw[->]  (t_1) edge (t_2) ;
% \draw[->]  (t_2) edge (t_3) ;
% \end{tikzpicture}
% \end{center}
% In fact, predictions $\prediction_{jmp}$ that contain
% $t_2 \mapsto v$ for arbitrary $v$ may redirect the control flow to arbitrary gadgets.
Retpoline has the effect of  transforming  indirect jumps at address
$a_2$ of Example~\ref{example:spectre:v2} as:\\
\begin{tikzpicture}[node distance=3cm,auto,>=latex']
\pomsetstyle
\node[name=a_2]{$a_2$};
\picloadT[right =.3cm of a_2]{t_{21}}{\Regs}{sp}
\picexpT[right of = t_{21}]{t_{22}}{t_{21} - 4}
\picstoreT[right of = t_{22}]{t_{23}}{\Regs}{sp}{t_{22}}
\picexpT[below = \pomsetnewline of t_{21}]{t_{24}}{a_{3}}
\picstoreT[right of = t_{24}]{t_{25}}{\Locs}{t_{21}}{t_{24}}
\picstoreT[right of = t_{25}]{t_{26}}{\pc}{}{b_1}
\draw[->]  (t_{21}) edge (t_{22}) ;
\draw[->]  (t_{22}) edge (t_{23}) ;
\draw[->]  (t_{21}) edge (t_{25}) ;
\draw[->]  (t_{24}) edge (t_{25}) ;
\end{tikzpicture}\\
\begin{tikzpicture}[node distance=3.5cm,auto,>=latex']
\pomsetstyle
\node[name=a_1]{$a_3$};
\picstoreT[right =.3cm of a_1]{t_{31}}{\Pc}{}{a_3}
\end{tikzpicture}\\
\begin{tikzpicture}[node distance=3cm,auto,>=latex']
\pomsetstyle
\node[name=b_1]{$b_1$};
\picloadT[right =.3cm of b_1]{t_{41}}{\Regs}{sp}
\picexpT[right of = t_{41}]{t_{42}}{t_{41} + 4}
\picloadT[below = \pomsetnewline of t_{41}]{t_{43}}{\Locs}{p}
\picexpT[right of = t_{43}]{t_{44}}{t_{43}}
\picstoreT[right of = t_{42}]{t_{45}}{\Locs}{t_{42}}{t_{44}}
\picstoreT[right of = t_{44}]{t_{46}}{\Pc}{}{b_2}
\draw[->]  (t_{41}) edge (t_{42}) ;
\draw[->]  (t_{42}) edge (t_{45}) ;
\draw[->]  (t_{43}) edge (t_{44}) ;
\draw[->]  (t_{44}) edge (t_{45}) ;
\end{tikzpicture}\\
\begin{tikzpicture}[node distance=3cm,auto,>=latex']
\pomsetstyle
\node[name=b_2]{$b_2$};
\picloadT[right =.3cm of a_1]{t_{51}}{\Regs}{sp}
\picexpT[right of = t_{51}]{t_{52}}{t_{51} + 4}
\picstoreT[right of = t_{52}]{t_{53}}{\Regs}{sp}{t_{52}}
\picloadT[below = \pomsetnewline of t_{51}]{t_{54}}{\Locs}{t_{52}}
\picexpT[right of = t_{54}]{t_{55}}{t_{54}}
\picstoreT[right of = t_{55}]{t_{56}}{\Pc}{}{t_{55}}
\draw[->]  (t_{51}) edge (t_{52}) ;
\draw[->]  (t_{52}) edge (t_{53}) ;
\draw[->]  (t_{52}) edge (t_{54}) ;
\draw[->]  (t_{54}) edge (t_{55}) ;
\draw[->]  (t_{55}) edge (t_{56}) ;
\end{tikzpicture}\\
Instruction at $a_2$ calls a \emph{trampoline} starting at address $b_1$ and
instruction at $a_3$ loops indefinitely.
The first instruction of the trampoline overwrites the return address on the stack with
the value of at address $p$ and its second instruction at $b_2$
returns.

We leverage our model to analyze the effectiveness of Retpoline for
indirect jumps.
Since address $b_1$ is known at compile time, $t_{26}$ does not trigger
jump target prediction.
While executing the trampoline, the value of $t_{55}$ may be mispredicted,
especially if the load from $p$ has not been executed and the store $t_{45}$
is postponed.
However, $b_2$ is a \verb|ret|, hence
the value of $t_{55}$ is predicted via $\prediction_{RSB}$. Since there is no
call between $a_1$ and $b_2$, then prediction can only assign the address $a_3$ to
$t_{55}$ (i.e., $\proj{\prediction_{RSB}}{t_{55}} \subseteq \{t_{55} \rightarrow a_3\}$).
Therefore, the RSB entry generated by $a_2$ is used
and mispredictions are captured with the infinite loop in $a_3$. Ultimately, when
the value of $t_{55}$ is resolved, the correct return address is used
and the control flow is redirected to the value in of $*p$, as expected.

\subsection{ARM Speculative Store Bypass Safe}
The specification of proposed  hardware countermeasures  oftentimes comes with no precise semantics and is ambiguous. 
InSpectre provides a ground to formalize the behavior of  hardware
mechanisms like memory fences.
For instance, ARM introduced  the Speculative Store
Bypass Safe (SSBS) configuration to prevent store bypass
vulnerabilities. The specification of SSBS~\cite{ssbs} is:
\emph{
Hardware is not permitted to load \dots speculatively, in a
manner that could \dots give rise to a \dots side
channel, using an address derived from a register value that has been
loaded from memory \dots (L) that speculatively
reads an entry from earlier in the coherence order from that location
being loaded from than the entry generated by the latest store (S) to
that location using the same virtual address as L.
}
% \begin{quote}
% Hardware is not permitted to load or store speculatively, in a
% manner that could practically give rise to a cache timing side
% channel, using an address derived from a register value that has been
% loaded from memory using a load instruction (L) that speculatively
% reads an entry from earlier in the coherence order from that location
% being loaded from than the entry generated by the latest store (S) to
% that location using the same virtual address as L.
% \end{quote}

We formalize SSBS as follows.
Let $\newstate = (\Inst, \storage, \commits, \decodes, \spec, \guesses)$  and $\ass{c}{t}{\load{\restype}{t_a}} \in
\newstate$. 
If $\newstate \triplestep{l}{}  \newstate'$, $\fundefined{\newstate}{t}$, and 
$\fdefined{\newstate'}{t}$,
then
for every $t' \in \sources(t,\newstate)$, if $\newstate(t') \neq \newstate(t_a)$
then $t' \not \in \guesses$.

The reason why SSBS prevents Spectre-STL is simple. The rule
forbids the execution of a load $t$ if any address used to 
identify the last store affecting $t_a$  has been
predicted to differ from $t_a$.
% For instance, in the example of Section~\ref{sec:dep} SSBS stalls the execution of $t_{42}$
% while one of the previous address is guessed: i.e. $\{t_{11}, t_{21},
% t_{31}\} \cap \guesses \neq \emptyset$.
Observe that SSBS does not prevent Spectre-STL-D, where, in order to
enable store forward,  the CPU predicts that a store
affects the same address of a subsequent load.

\subsection{Implicit serialization to prevent Spectre-PHT}\label{sec:spectre:cmov}
\todo{Explain in Spectre-PHT that we only speculate if there is a
  memory operation}
An alternative approach to prevent Spectre-PHT is to use instructions
that introduce implicit serialization~\cite{cmov}. For instance, the
following variation of the program of Section~\ref{appendix:pht}
prevents Spectre-PHT in existing Intel CPUs:
\begin{lstlisting}[mathescape=true]
$a_1: r_1 = A_1.size;$
$a_2: if\; (r_0 < r_1)$
$a'_3: \quad\ \  f = (r_0 \ge r_1)$ // cmp
$a''_3: \quad\  cmov f, r_0, 0$
$a'''_3:  \quad y = A_2[A_1[r_0]];$
\end{lstlisting}
Intuitively, this modification forces the access to 
$A_1[0]$ in case of misprediction.
The program can be translated to MIL as follows (we only report the
modified instructions):
\\
\begin{tikzpicture}[node distance=3cm,auto,>=latex']
\pomsetstyle
\node[name=a'_3]{$a'_3$};
\picloadT[right =.3cm of a'_3]{t'_{31}}{\Regs}{r_0}
\picexpT[right of = t'_{31}]{t'_{33}}{t'_{31} \ge t'_{32}}
\picloadT[right of = t'_{33}]{t'_{32}}{\Regs}{r_1}
\picstoreT[below = \pomsetnewline of t'_{33}]{t'_{34}}{\Regs}{f}{t'_{33}}
\picstoreT[below = \pomsetnewline of t'_{32}]{t'_{35}}{\Pc}{}{a''_3}
\draw[->]  (t'_{31}) edge (t'_{33}) ;
\draw[->]  (t'_{32}) edge (t'_{33}) ;
\draw[->]  (t'_{33}) edge (t'_{34}) ;
\end{tikzpicture}
\\
\begin{tikzpicture}[node distance=3cm,auto,>=latex']
\pomsetstyle
\node[name=a''_3]{$a''_3$};
\picloadT[right =.3cm of a''_3]{t''_{31}}{\Regs}{f}
\picstore[right of=t''_{31}]{t''_{32}}{t''_{31}=1}{\Regs}{r_0}{0}
\picstoreT[right =1.2cm of t''_{32}]{t''_{34}}{\Pc}{}{a'''_3}
\draw[->]  (t''_{31}) edge (t''_{32}) ;
\end{tikzpicture}\\
\begin{tikzpicture}[node distance=3cm,auto,>=latex']
\pomsetstyle
\node[name=a'''_3]{$a'''_3$};
\picloadT[right =.3cm of a'''_3]{t'''_{31}}{\Regs}{r_0}
\picloadT[right of = t_{31}]{t'''_{32}}{\Locs}{A_1.base + t'''_{31}}
\picloadT[below = \pomsetnewline of t_{32}]{t'''_{33}}{\Locs}{A_2.base + t'''_{32}}
\picstoreT[right of = t_{33}]{t'''_{34}}{\Regs}{r_0}{t'''_{33}}
\picstoreT[right of = t_{32}]{t'''_{35}}{\Pc}{}{a_4}
\draw[->]  (t_{31}) edge (t_{32}) ;
\draw[->]  (t_{32}) edge (t_{33}) ;
\draw[->]  (t_{33}) edge (t_{34}) ;
\end{tikzpicture}\\
Even if the $\prediction_{br}$ mispredicts the outcome of the conditional
branch (i.e. $t_{23} \mapsto 1$), the instruction in $a''_3$
introduces a data dependency between $t_{11}$ and $t'''_{32}$. In
fact, 
$\stract$ of $t'''_{31}$ includes $t''_{32}$ until $t''_{31}$;
has been executed; 
$\stract$ of $t''_{31}$ includes $t'_{34}$;
and $\stract$ of $t'_{32}$ includes $t_{12}$. Since all these names
(and intermediate dependencies via free names) are not condition of
program counter stores then they cannot be predicted by
$\prediction_{br}$ and their dependencies are enforced by the
semantics. In particular, when $t_{23}$ is mispredicted to
hold, $t''_{32}$ is executed after that $t_{11}$ has obtained the value from
the memory. This ensures that $t''_{32}$ sets $r_0$ to $0$ every time
a buffer over-read could occur. Therefore mispeculations generate the
observations $\dl{A_1.base + 0}$ and $\dl{A_2.base + A_1[0]}$, which
do not violate the security condition because $A_1$ and $A_2$ are
labeled public by the security policy.

%%% Local Variables:
%%% mode: latex
%%% TeX-master: "ccs2020-main"
%%% End:
